# Supplementary material for: Full-Field Interferometric Imaging of Propagating Action Potentials
Source: arXiv:1807.03269 ancillary file (2018-07-03)
Supplement: Supplementary file 1 [file supplementary-information.pdf]

# Supplementary Information

## Supplementary Videos

**Video 1:** Spike-triggered average (STA) phase movie of two action potentials propagating across the field of view (FOV) of $159 \times 99\ \mu m^2$.

**Video 2:** Comparison of two STA phase movies based on optically- and electrically- detected spikes.

# Supplementary Figures

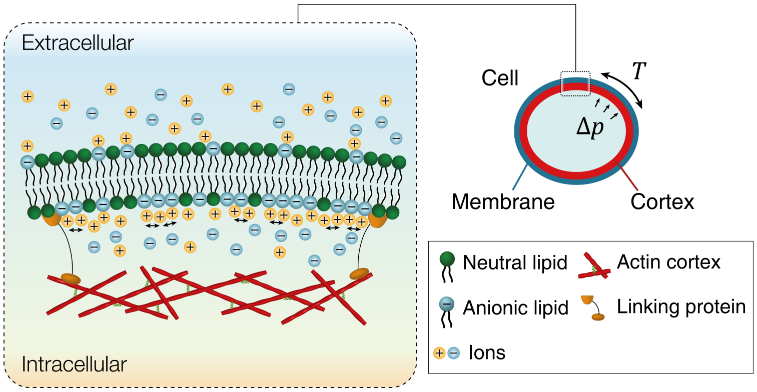


**Figure S1.** The shape of a cell is determined by the balance of hydrostatic pressure $\Delta p$, cytoskeleton strain and membrane tension $T$, which depends on concentration of ions along its surface. Upon depolarization, increased surface tension of the lipid bilayer leads to cell deformation.

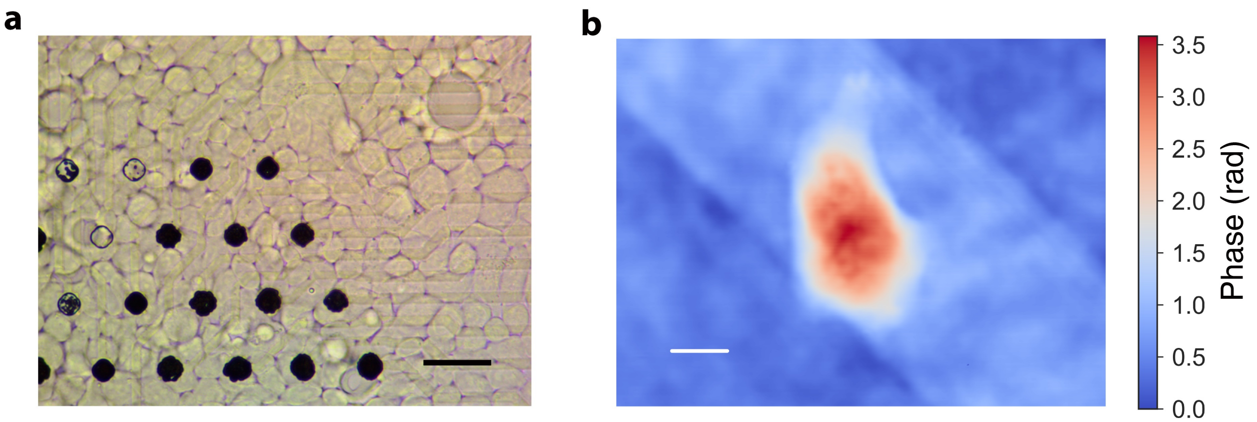


**Figure S2.** Bright-field and phase images of the spiking HEK-293 cells. (a) Bright-field image via 60× objective of cells plated on 61-electrode MEA with transparent indium tin oxide (ITO) leads. Solid circles are Pt-coated electrodes, while hollow circles indicate electrodes that failed to be platinized. Scale bar: 30 $\mu$m. (b) Phase image of a spiking HEK cell above an ITO wire. Scale bar: 10 $\mu$m.

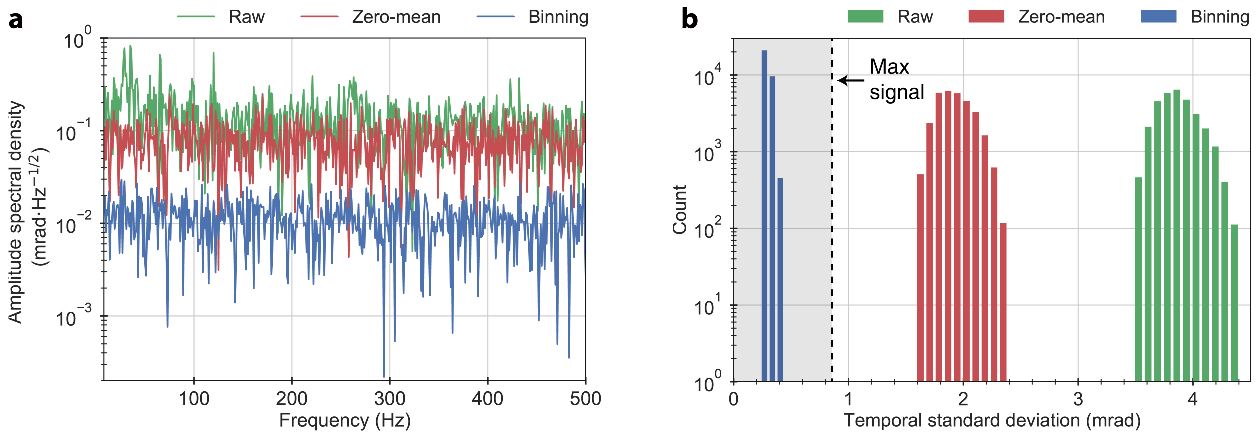


**Figure S3.** Noise reduction for single-spike detection. (a) Spectral density of the phase noise in a single pixel. Raw phase data is shown in green. Background subtraction (red) suppresses the effect of mechanical vibrations and variations in laser intensity, and reduces the phase noise close to the shot-noise limit. Binning 50 frames into one further reduces the noise to $\sim 10^{-2}$ mrad$\cdot$Hz$^{-1/2}$. (b) Temporal distribution of noise (standard deviation) in all pixels. With background removal and binning of 50 frames (blue), noise drops below the maximum signal level.
